# Supplementary material for: Observation of enhanced free-electron radiation from photonic flatband resonances
Source: arXiv:2110.03550 ancillary file (2021-10-07)
Supplement: Supplementary file 1 [file supplementary.pdf]

# Supplementary Information
# Observation of enhanced free-electron radiation from photonic flatband resonances

Yi Yang,[1,*] Charles Roques-Carmes,[1,*] Steven E. Kooi,[2] Haoning Tang,[3] Justin Beroz,[1] Eric Mazur,[3] Ido Kaminer,[4] John D. Joannopoulos,[1,2] and Marin Soljačić[1,2]

[1]*Research Laboratory of Electronics and Department of Physics, Massachusetts Institute of Technology, Cambridge, Massachusetts 02139, USA*

[2]*Institute for Soldier Nanotechnologies, Massachusetts Institute of Technology, Cambridge, Massachusetts 02139, USA*

[3]*Harvard John A. Paulson School of Engineering and Applied Sciences, Harvard University, Cambridge Massachusetts 02138, USA*

[4]*Department of Electrical and Computer Engineering, Technion–Israel Institute of Technology, 32000 Haifa, Israel*

## CONTENTS

S1. Point and line degeneracies between electron surface and photonic band 1

S2. Radiation experimental setup 2

S3. Band structure measurements 3

S4. Beam diameter and divergence 4

S5. Analytical methods 5

S6. Numerical methods 8

S7. Enhancement 8

S8. Shift and broadening of enhancement 9

References 12

## S1. POINT AND LINE DEGENERACIES BETWEEN ELECTRON SURFACE AND PHOTONIC BAND

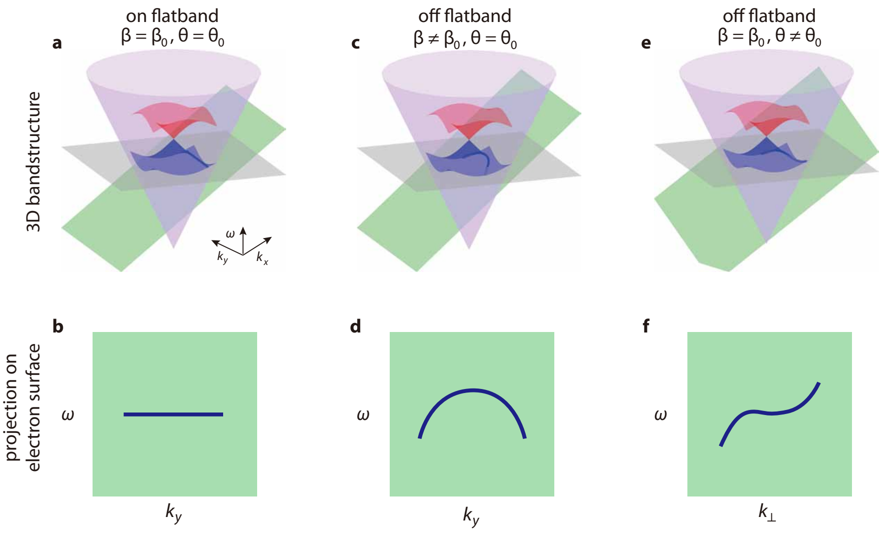


**Figure S1**. **Achieving the interaction between the electron surface (green) and the flatband requires the control of the electrons' velocity $\beta = v/c$ and their in-plane twist angle $\theta$ with photonic crystal slab. a-b.** At a certain velocity $\beta_0$ and a certain twist angle $\theta_0$, the intersection (solid blue line) becomes flat and thus forms a line degeneracy with the associated isofrequency surface, which substantially enhances electron-light interaction and free-electron radiation. In our case, $\theta_0 = 0$ because the flatband is perpendicular to the $\Gamma - X$ direction. **c-d.** At other velocities $\beta \neq \beta_0$, the intersection on the electron surface (green) is non-flat, rendering point degeneracies with an isofrequency surface (grey). **e-f.** At other twist angles $\theta \neq \theta_0$, free electrons and the PhC slab form a moiré systems, resulting in a relative twist between the photonic bands and the electron surface. Therefore, the intersection also becomes non-flat. The light cone is in purple and photonic bands are shown in red and blue. In f, $k_\perp = |-k_x \sin\theta\hat{x} + k_y \cos\theta\hat{y}|$.

## S2. RADIATION EXPERIMENTAL SETUP

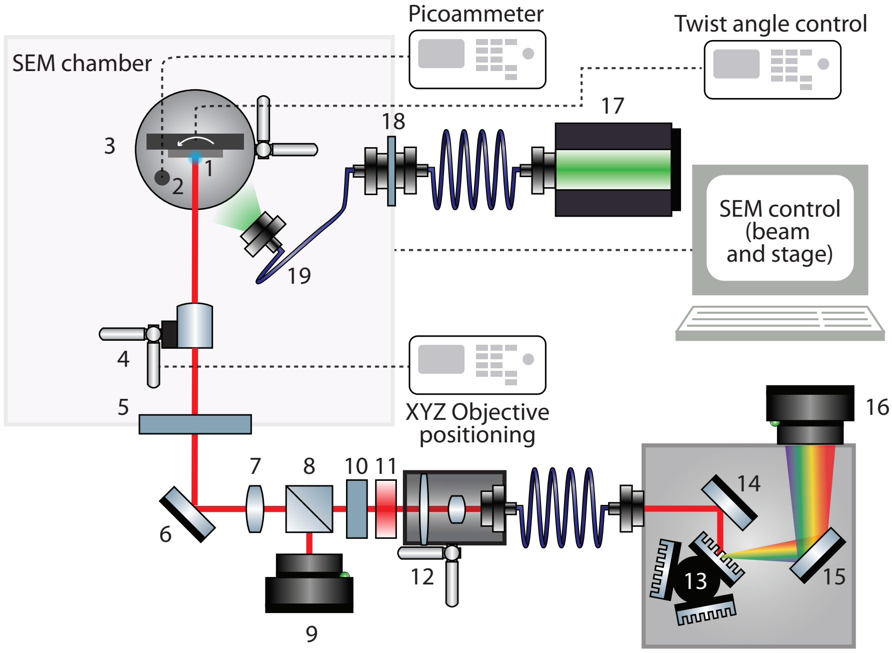


**Figure S2**. **Radiation experimental setup.** Inside SEM chamber: 1: Electron beam interacting with sample; 2: Faraday cup, connected to external picoammeter, measuring incident current. 3: 6-axis, fully eucentric stage, controlled by SEM control. Twist angle rotation stage. 4: XYZ objective stage. 5: X-ray blocking window. Outside SEM chamber: 6: Mirror. 7: Tube lens. 8: Beam splitter. 9: CCD Camera, imaging sample surface. 10: polarizer (optional). 11: filter. 12: XYZ cage assembly with two focusing lenses and a fiber-coupling. Inside spectrometer: 13: Grating turret. 14, 15: (Focusing) Mirrors. 16: Spectrometer InGaAs linear array. Green laser feedthrough alignment arm: 17: Green laser source. 18: Fiber-coupling feedthrough, vacuum compatible. 19: Fiber output illuminating sample.

The radiation experimental setup, shown in Figure S2, is based on an upgraded modified Scanning Electron Microscope (SEM) setup (an early version of which being reported in [S1–S4]). We provide additional information on the various components of the setup, that are not shown in the main text. The polarization-insensitive beamsplitter (Element 8) sends part of the signal to a visible CCD Camera (Hamamatsu). The combination of Elements 4 (objective), 7 (tube lens), and 9 (camera) creates an image of the sample's surface, so the location of the electron beam interaction with the sample can be visualized. The CCD provides the images shown in Section S5 and is used for optical alignment purposes. Elements 17-19 are used to scatter light off from the surface of the sample, also for alignment purposes. A set of two lenses is used (Element 12) to focus the optical signal into the fiber input feeding the spectrometer (Elements 13-16). The spectrometer is comprised of a fiber coupling into a slit, a grating turret (Element 13), and a mirror focusing the signal on an infrared InGaAs linear array (Element 16).

### A. SEM Control

The SEM beam current, voltage, working distance, spot size, and stage positioning are controlled in part with the Caesium Software provided by Applied Beams LLC (Oregon). Adjustment knobs outside the SEM chamber allow to align the emitter, apertures, focusing lenses, stage rotation and tilts.

### B. Objective positioning

The XYZ positioning and tilt angle alignment of the objective (Element 4) is realized with a homemade motorized stage. The three motors are controlled through a computer interface outside the SEM chamber.

Each motor is connected to an outside controller through a vacuum-preserving electronic connector.

### C. Twist angle control

A rotational degree of freedom, angle $\theta$, to the sample holder was implemented to manipulate the in-plane twist angle between the electron beam and the PhC slab. The twist angle is adjusted with a piezo motor tilt stage (range $\pm 5°$) controlled outside the SEM chamber via an electronic feedthrough. The twist angle can be read with accuracy $\pm 0.5°$ by looking through a SEM window flange.

### D. Measurement protocol

Each data point (shown e.g. in Fig. 3d-f and Fig. 3a-b) was acquired over 10s (10 averaged acquisitions which are each 1s long). Error bars, when applicable, are calculated as the standard deviation over the 10 acquisitions. For each measurement, the electron beam was positioned around the center of the camera field of view, after the XYZ position of the collection objective was optimized for maximum collection (using the motorized objective stage). The electron beam is slightly shifted off-center in the vertical direction in order to obtain maximum contrast of the peak with respect to the background at every measured energy. Background was measured as the signal from an unpatterned (unetched) sample from the same wafer. The location of the sample under electron beam exposure was regularly moved in order to reduce long-term beam exposure optical degradation of the sample.

## S3. BAND STRUCTURE MEASUREMENTS

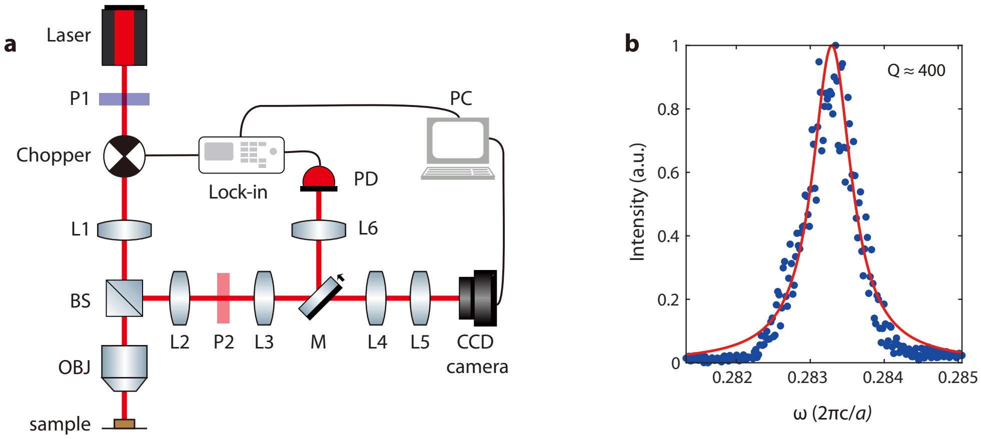


**Figure S3**. **Band structure measurements. a.** Optics setup. P, polarizer; L, lens; BS, beam splitter; OBJ, objective; M, flip mirror; PD, photodetector. **b.** Measured quality factor at the flatband.

We used Fourier spectroscopy (Fig. S3a) to determine the band structure of the photonic crystal (PhC) slab. The photonic crystal slab was illuminated with a polarized, collimated, tunable (1500 – 1630 nm) laser beam focused by a near-infrared objective (20X Mitutoyo Plan Apo NIR Infinity Corrected Objective, NA= 0.4). For a given wavelength, we adjusted the incidence angle to match the momentum of a particular resonant pump mode. Light from that specific resonant mode was then scattered into other modes at the same frequency, as enabled by fabrication disorder. Their far-field radiation was thus resolved in momentum space as isofrequency contours. We removed the incident laser beam using a pair of crossed polarizers (P1 and P2) and then imaged the contours through a $4f$ system onto a CCD camera.

To measure the quality factor of the device, we placed a pinhole in the Fourier plane after the first $4f$ system (L2 and L3). The diameter of the pinhole is 150 µm, yielding a momentum resolution of

$\delta k \approx 0.0015 \cdot 2\pi/a$. The pinhole selected specific $k$-points on the isofrequency contours and passed light to a photodiode. The photodiode was connected to a lock-in amplifier which was synchronized with a 1 kHz chopper placed in front of the incident laser beam. We could vary the pinhole position and record the scattered light from the lock-in amplifier to obtain the quality factor at various frequencies. The measured total quality factor of the PhC was $Q_\mathrm{o} \approx 400$ in the vicinity of the flatband in this optical characterization.

## S4. BEAM DIAMETER AND DIVERGENCE

We estimate the electron beam diameter $D$ and divergence angle $\alpha$ analytically and measure the beam diameter experimentally, finding consistent results.

### A. Analytical estimate

The electron beam diameter $D$ can be estimated with the formula [S5–S7]

$$D^2 = D_0^2 + D_\mathrm{d}^2 + D_\mathrm{s}^2 + D_\mathrm{c}^2 = [C_0^2 + (0.6\lambda)^2]\alpha_\mathrm{p}^{-2} + \frac{C_\mathrm{s}^2\alpha_\mathrm{p}^6}{4} + \left(C_c\frac{\Delta E}{E}\right)^2 \alpha_\mathrm{p}^2. \tag{S1}$$

Here $D_0$ is the aberration-free Gaussian probe diameter, $D_\mathrm{d}$ corresponds to aperture diffraction, $D_\mathrm{s}$ corresponds to spherical aberration, and $D_\mathrm{c}$ corresponds to chromatic aberration. Our SEM uses a $LaB_6$ cathode, for the voltage regime (20–40 keV) we used, $D_\mathrm{d}$ and $D_\mathrm{c}$ are negligible [S5]

$$D^2 \approx D_0^2 + D_\mathrm{s}^2 = C_0^2\alpha_\mathrm{p}^{-2} + \frac{C_\mathrm{s}^2\alpha_\mathrm{p}^6}{4}, \tag{S2}$$

where

$$C_0 = \sqrt{4I/b\pi^2}, \tag{S3}$$

$b$ is the electron gun brightness, $I$ is the probe current, $\alpha_\mathrm{p}$ is the convergence semi-angle of the electron beam, and $C_\mathrm{s}$ is the spherical aberration coefficient. Compared to our previous setup [S1; S2] that used a Tungsten cathode, we work with a $LaB_6$ cathode in our current setup that provides us electron beam of higher quality. This is reflected in the increase of the brightness $b$ from $1 \times 10^5$ A/cm$^2$/sr (Tungsten) to $1 \times 10^6$ A/cm$^2$/sr ($LaB_6$) at 20 keV (see Table 2.1 in Ref. [S5]). The focal length (working distance) of our $LaB_6$ SEM is 50 – 70 mm, which corresponds to a spherical aberration coefficient $C_\mathrm{s} \approx 550 - 800$ mm considering the nearly linear relation between the working distance and $C_\mathrm{s}$ [S5; S7]. From Eq. S2, the minimum beam diameter possible and the associated optimal convergence semi-angle are

$$D_\mathrm{min} = (4/3)^{3/8}(C_0^3 C_\mathrm{s})^{1/4} \tag{S4}$$

and

$$\alpha_\mathrm{p}^\mathrm{opt} = (4/3)^{1/8}(C_0/C_\mathrm{s})^{1/4}, \tag{S5}$$

respectively. Fig. S4 shows the estimated beam diameter $D \approx 3 - 5.5$ µm and divergence angle $2\alpha_\mathrm{opt} \approx 2°$ based on Eqs.(S2) and (S5) under our experimental conditions. This divergence angle puts a limit to the attainable resolution of the in-plane, twist angle between electrons and the sample.

### B. Beam diameter measurements

We measured the electron beam waist experimentally, to confirm the analytical estimates provided in the previous section. The experimental setup is shown in Fig. S5: the electron beam was scanned across a sharp edge (razor blade). The scattered electrons were detected with a SEI (secondary electrons imaging)

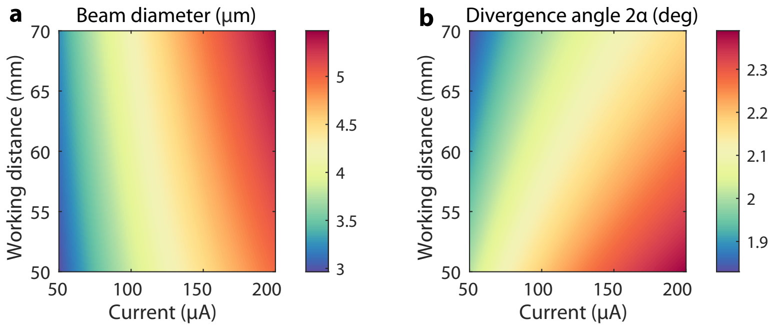


**Figure S4**. **Calculated beam diameter (a) and divergence angle (b) under experimental conditions.**

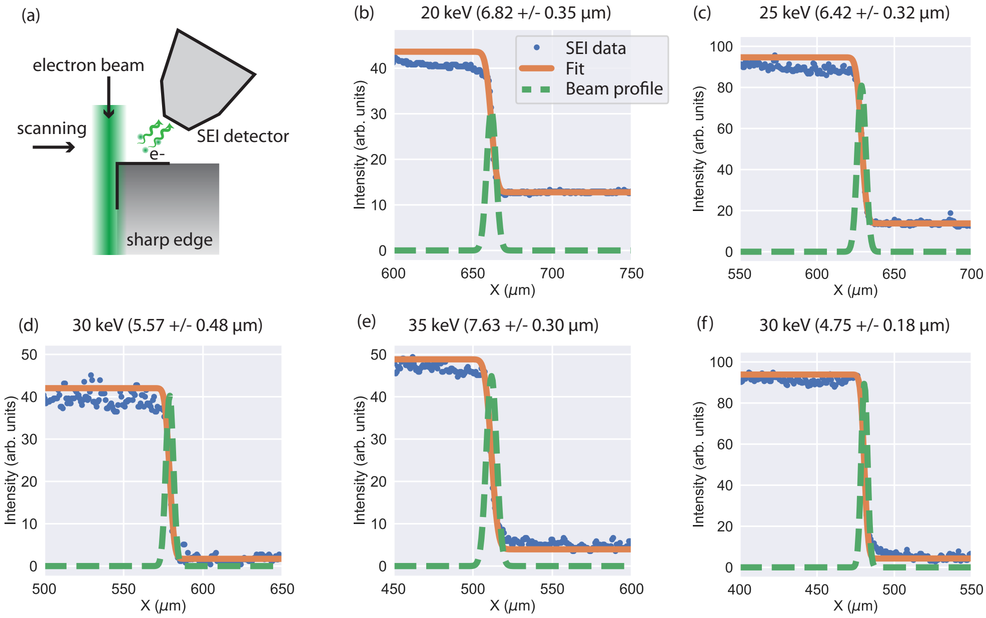


**Figure S5**. **Electron beam waist measurement. a.** Beam measurement setup. SEI: secondary electrons imaging. **b-f.** Beam measurement at indicated beam energy (keV). The measured beam FWHM (full width at half maximum) with uncertainty is indicated between parenthesis.

detector. An S-shaped signal was obtained as the electron beam went across the sharp edge. This signal was then fitted to an error function (integral of a Gaussian function) to extract the beam FWHM (full width at half maximum) and the corresponding beam profile. The measured beam FWHMs were in the range 4.75 – 7.63 μm and varied with the electron beam energy. The measured values are consistent with the analytical models.

## S5. ANALYTICAL METHODS

We are able to semi-analytically predict the collected radiation intensity from the PhC slab based on the upper limit theory of spontaneous free-electron radiation [S1] and ray tracing in momentum space. The collected radiation intensity signal $S(\beta, \omega)$ can be decomposed as a product

$$S(\beta, \omega) \propto \Gamma(\beta, \omega, d) R(\beta, \omega) \eta(\beta, \omega) \quad \text{(S6)}$$

among the radiation upper limit $\Gamma(\beta, \omega, d)$, the Lorentzian resonance $R(\beta, \omega)$, and the collection efficiency $\eta(\beta, \omega)$.

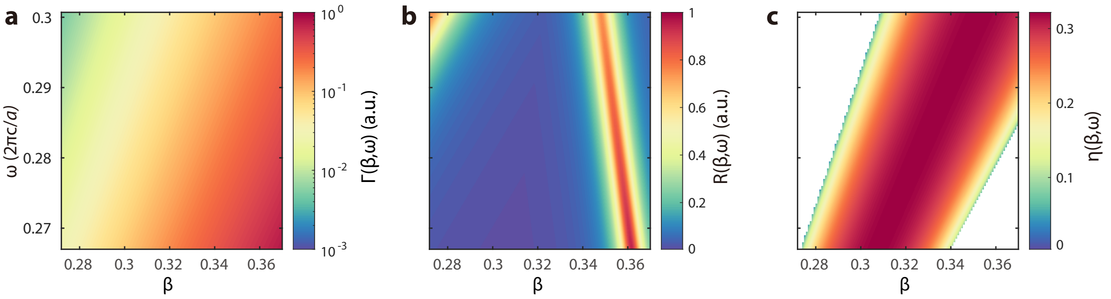


**Figure S6**. **Analytical results associated to Fig. 3b. a.** Free-electron radiation upper limit $\Gamma(\beta,\omega)$. **b.** Resonance trajectory $\omega_{\rm res}$. **c.** Collection efficiency $\eta(\beta,\omega)$.

We adopt the shape-independent upper limit formula [S1] to calculate $\Gamma(\beta,\omega,d)$ (Fig. S6a)

$$\Gamma(\beta,\omega,d) = \frac{\alpha}{8\pi c}\frac{|\chi|^2}{\mathrm{Im}\,\chi}\frac{L\mu}{\beta^2}\left[(\kappa_\rho d)K_0(\kappa_\rho d)K_1(\kappa_\rho d)\right], \tag{S7}$$

where $\alpha$ is the fine-structure constant, $L$ is the interaction length, $\mu$ is the opening angle of a minimal-sized sector that encloses the structure ($\mu=\pi$ for the PhC slab in our case), $\chi$ is the material susceptibility, $\kappa_\rho d = kd/\beta\gamma$ ($\gamma \equiv 1/\sqrt{1-\beta^2}$ being the Lorentz factor) is the impact parameter showing that the relevant length scale is set by the relativistic velocity of the electron and the Lorentz-contracted separation compared to the wavelength. In Eq. (S7), we choose the electron-PhC separation as half the beam diameter, i.e. $d = D/2 \approx 3.1\,\mu$m.

The resonance trajectory $\omega_{\rm res}(\mathbf{k})$ (Fig. S6b) can be obtained by taking the overlap between the electron surface $\omega=\beta k_\parallel$ (in the twisted angle $\theta=0°$ case, $k_\parallel = k_x$) with the calculated photonic band structure, i.e. $\omega_{\rm res}(\mathbf{k}) = \omega_{\rm PhC}(\mathbf{k}) \cap \beta k_\parallel$ [S8; S9]. The Lorentzian resonance profile can be expressed as

$$R(\beta,\omega) \propto \frac{1}{\partial\omega/\partial k_\perp}\frac{1}{\mathrm{Dist}\left[(\beta,\omega),\omega_{\rm res}(\mathbf{k})\right]+\gamma^2}, \tag{S8}$$

where the first fraction accounts for the enhancement from the band flatness [S10] and the second fraction accounts for the enhancement from the quality factors. In the electron radiation experiment, the measured quality factors $Q_{\rm e}^{\omega}$ were near 50 (e.g. see Fig. 3d and Fig. 4d), where the subscript e denotes 'electron' (cf. $Q_{\rm o}$ from the optical measurement in Sec. S3) and the superscript $\omega$ denotes frequency as in the usual definition of quality factors. Meanwhile, another type of quality factor $Q_{\rm e}^{\mathbf{k}}$, in terms of momentum, also contributes here because of the electron beam is not perfectly collimated but has a particularly relevant, in-plane velocity spread. Since we were able to simultaneously excite both $s-$ and $p-$polarized modes with electron beams of a single energy, this indicates a velocity spread $\gtrsim 5\%$ (Fig. 4a and d), i.e. $Q_{\rm e}^{\mathbf{k}} \lesssim 20$. Since $Q_{\rm e}^{\omega}$ and $Q_{\rm e}^{\mathbf{k}}$ are close in our radiation measurements, we adopt the Euclidean distance (Dist in Eq. S8) between a given parameter $(\beta,\omega)$ and the resonance trajectory $\omega_{\rm res}(\mathbf{k})$ to take account of both $Q_{\rm e}^{\omega}$ and $Q_{\rm e}^{\mathbf{k}}$.

The collection efficiency $\eta(\beta,\omega)$ (Fig. S6c) can be obtained from geometrical optics. In our setup, The electron beam propagated at a small grazing angle and thus created a region that emitted most radiation in the PhC slab. We were able to control the relative translation between the objective and the light emitting region to preferentially collect radiations toward certain directions. Recall the Smith–Purcell relation for the first-order radiation

$$\sin\psi = 1/\beta - 1/\omega, \tag{S9}$$

where $\psi$ is the polar angle from the surface normal on the longitudinal surface (i.e. surface formed by the electron velocity and the surface normal of the PhC slab) and we approximate radiation in the transverse direction, at each $\psi$, to be isotropic. Let $\omega_0$ be the frequency with maximal radiation enhancement and $k_0$ the associated in-plane longitudinal momentum, their polar angle $\psi_0 = \sin^{-1} k_0/\omega_0$ [also see Eq. (2)] thus becomes the chief ray angle of the objective (i.e. radiation at $\omega_0$ passes the center of the objective), which corresponds to a horizontal translation $x_0 \propto \sqrt{1-\mathrm{NA}^2}\tan\psi_0$. The collection efficiency at certain $\omega$ thus

corresponds to the angle enclosed by its associated chord (red bold line in Fig. S7) on the objective (blue in Fig. S7) in its transverse radiation plane (pink surface) :

$$\eta(\beta,\omega) = 2\tan^{-1}\frac{\sqrt{\mathrm{NA}^2-\left(1-\mathrm{NA}^2\right)(\tan\psi-\tan\psi_0)^2}}{\sqrt{1-\mathrm{NA}^2}/\cos\psi}. \tag{S10}$$

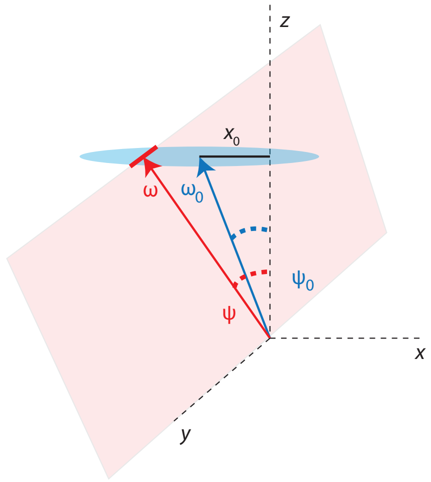


**Figure S7**. **Collection efficiency model.** Blue and red arrows indicates Smith–Purcell radiation at frequency $\omega_0$ and $\omega$ into angles $\psi_0$ and $\psi$. $\delta x$ is the translation in $x$ needed to collect maximal radiation at $\omega_0$. The collection efficiency for all $\omega$ can thus be determined via Eq. S10

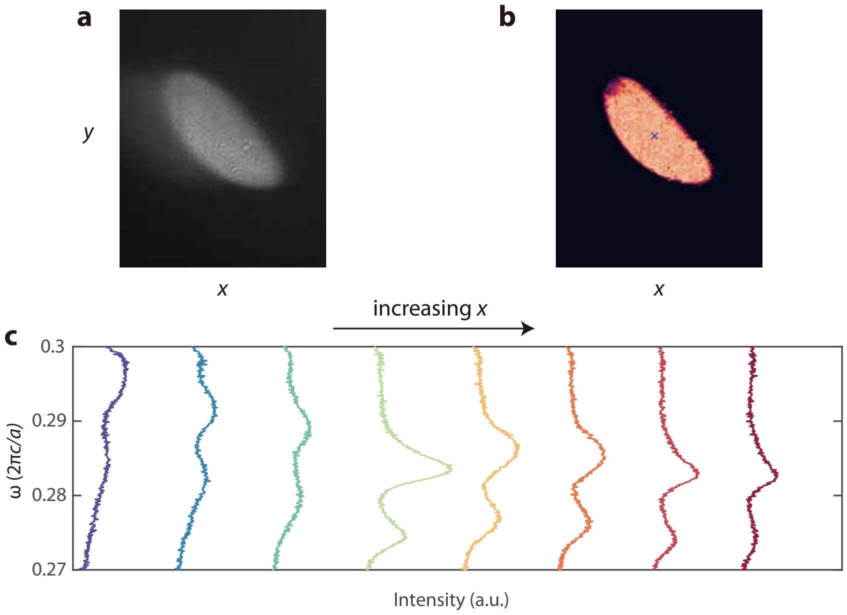


**Figure S8**. **Extraction of band structure by translating the position between the electron beam and the collection objective. a-b.** Raw (a) and processed (b) images from the CCD camera. The peak locations are calculated by imposing a binarization threshold filter to the raw CCD image, and measuring the mean value pixel value of the area with non-zero pixel value. **c.** Measured spectra by translating the beam along the $x$ direction in the field of view.

The same model for the collection efficiency also allows us to extract the longitudinal momentum $k_x^{\mathrm{exp}}$ for the band structure measurement from the radiation spectra by translating the electron beam in the field of

view. Since the collected radiation is limited by the numerical aperture, we can obtain the tunable chief polar angle $\psi_c$ as

$$\psi_c = \tan^{-1}\left(\tan\psi_0 + 2\delta_x \frac{\mathrm{NA}}{\sqrt{1-\mathrm{NA}^2}}\right), \tag{S11}$$

where $\delta_x$ is the relative translation of the center of the beam (Fig. S8a and b) along the $x$ direction, compared to the initial condition $x_0$. The longitudinal momentum in the experiment can thus be obtained as $k_x^{\mathrm{exp}} = \omega_0 \sin\psi_c$ for the spectra measured at each beam position (Fig. S8).

## S6. NUMERICAL METHODS

The photonic band structure in Fig. 3b is calculated using a finite-difference time-domain MEEP package [S11]. Numerical radiation probability is obtained via the frequency-domain calculation in the RF module in COMSOL Multiphysics. External fields of point electrons are modelled with line currents at each frequency. Radiation probability, under each electron velocity and at each frequency, is obtained by taking a surface integral of the Poynting vector above the photonic crystal slab. The wavevector component analysis in Fig. 3g is obtained by taking the Fourier transform of the real-space radiation. Since $k_x$ is determined by the electron velocity, $k_y$ and $k_z$ are constraint by the following relation

$$k_y^2 + k_z^2 = \sqrt{\omega^2 - k_x^2} = \frac{2\omega}{\beta} - \frac{\omega^2}{\beta^2\gamma^2} - 1 \tag{S12}$$

where $\beta = v/c$ is the electron velocity, and $\gamma = 1/\sqrt{1-\beta^2}$ is the Lorentz factor.

## S7. ENHANCEMENT

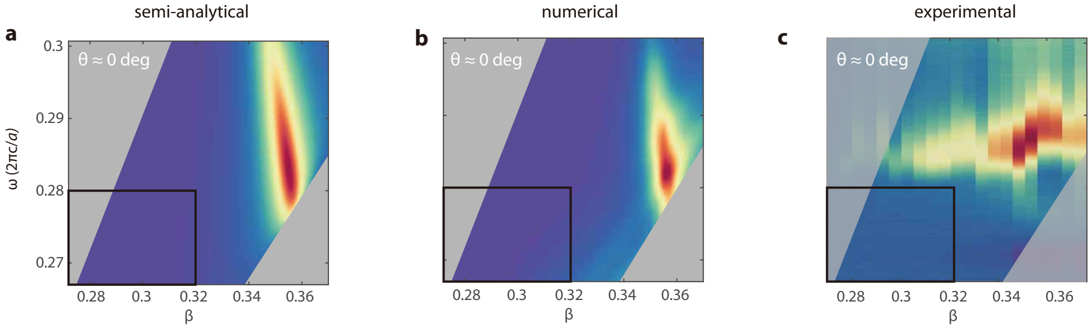


**Figure S9**. **Enhancement quantification. a.** Semi-analytical; **b.** Numerical; **c.** Experimental. Off-flatband regions are indicated by the black rectangles. a, b, and c are the same as the main text Fig. 3b, c, and d, respectively.

We use the ratio between the peak radiation and the average radiation in the off-flatband region to quantify the enhancement $\Lambda$:

$$\Lambda \sim \frac{\max\Gamma(\beta,\omega)}{\iint_S \Gamma(\beta,\omega)\,\mathrm{d}\beta\,\mathrm{d}\omega \,/\, \iint_S \mathrm{d}\beta\,\mathrm{d}\omega}, \tag{S13}$$

where $S = (\beta < 0.32, \omega < 0.28)$ is the off-flatband region (indicated by the black boxes in Fig. S9) in our measurement. $\Lambda$ reads 600, 500, and 100 for the semi-analytical, numerical, and experimental results, respectively (Fig. S9a–c). The enhancement from the semi-analytical calculation is slightly higher than the numerical enhancement because we only consider contributions from a single band in the semi-analytical treatment.

## S8. SHIFT AND BROADENING OF ENHANCEMENT

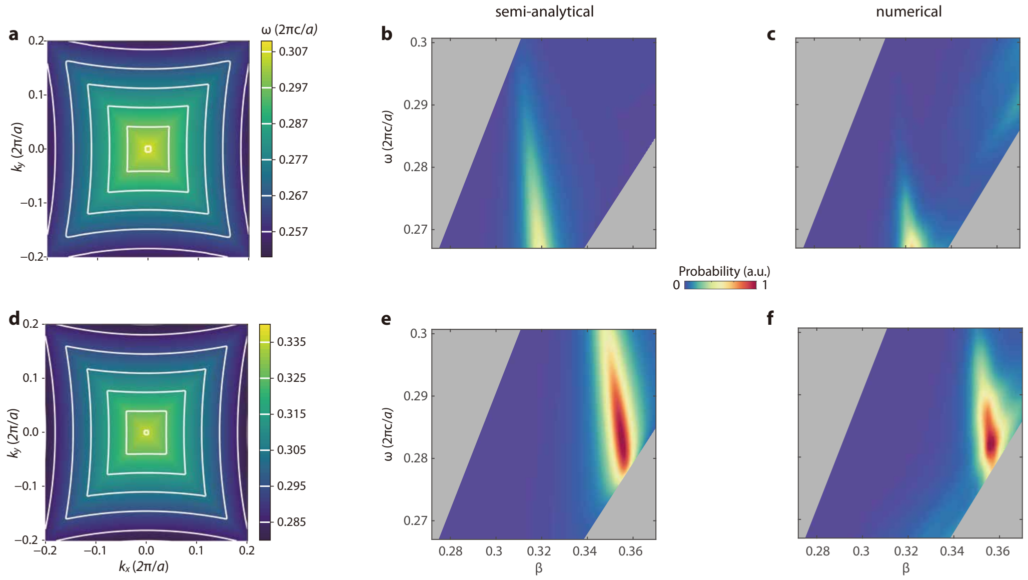


**Figure S10**. **Comparisons of the isofrequency contours of the PhC slab and the associated radiation spectra at zero twisted angle under** $\mathrm{Re}\, n_{\mathrm{Si}} = 3.5$ **(a-c) and** $\mathrm{Re}\, n_{\mathrm{Si}} = 3.2$ **(d-f).** b and e are calculated with the semi-analytical method (Sec. S5). c and f are calculated with the numerical method (Sec. S6). d, e, f are the same as Fig. 2b, Fig. 3b, and Fig. 3c, respectively. Shaded area in b, c, e, and f are outside the numerical aperture of the objective.

We observed resonance drift and broadening when comparing the measured radiation spectra (Fig. 3 and Fig. 4) with the optical characterizations (Fig. 2 and Fig. S3; under ambient conditions), which indicates changes of the optical responses of the sample under the active, 'electron-pumped' condition in the radiation measurements. The specific observations are

1. *Resonance shift along the velocity direction.* In our optics measurement, the flatband was characterized near $k_x \approx 0.08$ (Fig. 2d). Meanwhile, the free-electron radiation measurements indicated that the flatband was near $k_x \approx 0.17$ (Fig. 3d and Fig. 4d).
2. *Resonance broadening along the frequency direction.* The quality factor of the flatband was $\approx 400$ as in the optics measurement (Fig. S3b) while it reduced to $\approx 50$ in the radiation measurement (Fig. 4a; TM-like peak).
3. *Resonance broadening along the velocity direction.* In the measurement (Fig. 3d), the enhancement region is wider along the velocity direction compared with the theoretical predictions (Fig. 3b and c).

There are a few experimental uncertainties that could contribute to the observed shift and broadening:

1. *Increase of free carriers in silicon under electron bombardment.* In our experiment, the electron beam passed above and hit onto the PhC at a grazing angle ($\psi_e \approx 1°$). This results in an area $A \sim \pi D^2/4 \sin\psi_e \sim 10^{-5}\,\mathrm{cm}^2$ under electron bombardment. Recall that the current operates near $\sim 100\,\mu\mathrm{A}$, a high concentration of free carriers was injected into the light-emitting region of the silicon PhC slab and thus modified its optical responses.
2. *Temperature rise in materials.* Electron bombardment could also cause local temperature rise on the sample. *

---

* Since we did not observe melting of silicon (whose melting point of silicon is $\approx 1700\,\mathrm{K}$), the local temperature rise should be on the order of $10^2 - 10^3$ K, which translate into a linear refractive index shift $0.01 - 0.1$ at maximum considering silicon's thermal conductivity.

3. *In-plane momentum spread due to beam divergence* In contrast to point electrons in the modelling, the electron beam in the experiment was not perfectly collimated and had a divergence angle $\approx 2°$ (Sec. S4). The Coulomb repulsion from the charged area on the sample could cause additional divergence to the electron beam in the vicinity of the sample. †
4. *Surface oxidization.* Silicon forms an intrinsic oxide layer of a few nanometer thick under ambient conditions [S12]. The oxide layer may become thicker when the ultraviolet-ozone cleaning treatment was applied to the sample. ‡
5. *Surface contamination.* Remaining hydrocarbon molecules in the vacuum chamber could deposit onto and thus contaminate the sample surface during the radiation measurement. §

### A. Effective doping of silicon

Out of the uncertainties enumerated above, the key reason to the observed resonance shift and broadening along the frequency direction is the modifications to the optical properties of silicon under direct electron beam exposure and bombardment. Electrons could enter the PhC slab and caused an effective increase of the doping level in silicon, which rendered the material more conductive and optically absorptive.

The optical properties of silicon under different doping levels have been investigated previously (e.g. see Refs. [S14; S15] and references therein). Intuitively, the scenario could be understood by the Drude model. An increase of the doping level causes a decrease of $\mathrm{Re}\, n_{\mathrm{Si}}$ and an increase of $\mathrm{Im}\, n_{\mathrm{Si}}$ simultaneously (where $n_{\mathrm{Si}}$ is the refractive index of silicon), as consistent with the Drude picture. Compared to its intrinsic refractive index $\sim 3.5$ in the near-infrared regime, $n_{\mathrm{Si}}$ could reduce to $\sim 2 + 1\mathrm{i}$ near $2\,\mu\mathrm{m}$, which is highly metallic, under a high doping concentration $\sim 10^{21}\,\mathrm{cm}^{-3}$ [S14].

In our radiation measurement inside a modified scanning electron microscope, the instantaneous refractive index of our sample under simultaneous beam exposure could not be measured in-situ, which makes it challenging for theoretically calculating the associated radiation spectra shown in Fig. 3a and b. In these calculations shown in the main text, alternatively, we choose $n_{\mathrm{Si}} = 3.2 + 0.03\mathrm{i}$, which corresponds to an effective doping concentration $10^{20} – 10^{21}\,\mathrm{cm}^{-3}$ based on previous studies [S14; S15]. The material dispersion of the index of silicon is neglected because the relevant frequency window in our measurement is narrow.

We compare the calculated isofrequency contours under $\mathrm{Re}\, n_{\mathrm{Si}} = 3.5$ and $\mathrm{Re}\, n_{\mathrm{Si}} = 3.2$ in Fig. S10a and d. Under a smaller refractive index, the band moves toward higher frequencies. The frequency window in our measurement, $\omega \sim 0.27 – 0.3$, thus possesses larger in-plane momenta. Such modifications to the band structure are reflected in the calculated radiation spectra (Fig. 3b, c, e, and f). As shown in both the semi-analytical (Fig. S10b and e) and numerical (Fig. S10c and f) results, the 'resonant' velocity, which corresponds to the peak enhancement of radiation, moves from $\beta \approx 0.32$ ($\mathrm{Re}\, n_{\mathrm{Si}} = 3.5$) to $\beta \approx 0.35$ ($\mathrm{Re}\, n_{\mathrm{Si}} = 3.2$).

### B. Enhancement broadening along the velocity direction

Two major reasons could explain the observed enhancement broadening along the velocity axis in Fig. 3.

1. *Temporal and spatial fluctuation of carriers.* As can be seen from Fig. 3b, c, e, and f, if one adiabatically modifies $\mathrm{Re}\, n_{\mathrm{Si}}$, the enhancement region forms a trajectory in the $(\beta, \omega)$ parameter space.

---

† The beam divergence, although relevant to the broadening of the enhancement, should contribute negligibly to the resonance shift.

‡ As the surface oxidization is self-limiting, the oxide thickness of silicon is still less than tens of nanometers even under hours of high-temperature oxidization process [S13], compared to which the oxidization in our case should be much milder.

§ The accumulation of surface contamination occurred at a much longer time scale than the other factors listed above and our data collection.

This trajectory of enhancement explains the broadening of the enhancement region along the electron velocity direction $\beta$ (compare Fig. 3d with Fig. 3b and c). In our theoretical calculations, we assume a simple constant modification to $n_{\mathrm{Si}}$ as described above. However, in the experiment, $n_{\mathrm{Si}}$ had extra temporal and spatial dependence which could stem from a variety of factors including the density distribution of the electron beam, the Coulomb repulsion between the electron beam and the charged sample surface, and the diffusion of electrons inside the sample. Therefore, the theoretical treatment—constant modification to $n_{\mathrm{Si}}$—should be understood as the zeroth-order expansion of $n_{\mathrm{Si}}(\mathbf{r}, t)$. The fluctuation of $n_{\mathrm{Si}}$, in both space and time, contributed to the broadening of the enhancement region along the velocity $\beta$ direction in our measurements.

2. *Concurrent radiation pathways.* In our experiment, Concurrent radiation pathways could form a broadened measurement background that is not captured by the theoretical treatments (Fig. 3b and c), since they focus only on Smith–Purcell radiation.

   Because the electron beam was launched at a nonzero grazing angle, electrons also impinged onto the sample. Therefore, aside from Smith–Purcell radiation, other radiation pathways [S16], like incoherent cathodoluminescence and transition radiation, could occur simultaneously. These types of radiation could also get enhanced by the flatband with less sensitivity on the choice of electron velocity because of their localized nature (in contrast to the extended nature of Smith–Purcell radiation).

## References


* yiy@mit.edu; chrc@mit.edu; Y. Y. and C. R.-C. contributed equally to this work.

[S1] Y. Yang, A. Massuda, C. Roques-Carmes, S. E. Kooi, T. Christensen, S. G. Johnson, J. D. Joannopoulos, O. D. Miller, I. Kaminer, and M. Soljačić, Nature Physics **14**, 894 (2018).

[S2] C. Roques-Carmes, S. E. Kooi, Y. Yang, A. Massuda, P. D. Keathley, A. Zaidi, Y. Yang, J. D. Joannopoulos, K. K. Berggren, I. Kaminer, *et al.*, Nature communications **10**, 1 (2019).

[S3] A. Massuda, C. Roques-Carmes, Y. Yang, S. E. Kooi, Y. Yang, C. Murdia, K. K. Berggren, I. Kaminer, and M. Soljačić, ACS Photonics **5**, 3513 (2018).

[S4] I. Kaminer, S. Kooi, R. Shiloh, B. Zhen, Y. Shen, J. López, R. Remez, S. Skirlo, Y. Yang, J. Joannopoulos, and M. Soljačić, Phys. Rev. X **7**, 011003 (2017).

[S5] L. Reimer, *Scanning electron microscopy: physics of image formation and microanalysis*, Vol. 45 (Springer-Verlag, 1998).

[S6] J. Goldstein, D. E. Newbury, D. C. Joy, C. E. Lyman, P. Echlin, E. Lifshin, L. Sawyer, and J. Michael, *Scanning Electron Microscopy and X-ray Microanalysis* (Springer Science & Business Media, 2012).

[S7] A. Khursheed, *Scanning electron microscope optics and spectrometers* (World scientific, 2011).

[S8] C. Luo, M. Ibanescu, S. G. Johnson, and J. Joannopoulos, Science **299**, 368 (2003).

[S9] S. Yamaguti, J.-i. Inoue, O. Haeberlé, and K. Ohtaka, Phys. Rev. B **66**, 195202 (2002).

[S10] C. Kremers, D. N. Chigrin, and J. Kroha, Physical Review A **79**, 013829 (2009).

[S11] A. F. Oskooi, D. Roundy, M. Ibanescu, P. Bermel, J. D. Joannopoulos, and S. G. Johnson, Computer Physics Communications **181**, 687 (2010).

[S12] M. Morita, T. Ohmi, E. Hasegawa, M. Kawakami, and M. Ohwada, Journal of Applied Physics **68**, 1272 (1990).

[S13] H. Cui, C. Wang, and G. Yang, Nano letters **8**, 2731 (2008).

[S14] S. Basu, B. J. Lee, and Z. M. Zhang, Journal of Heat Transfer **132**, 023301 (2010).

[S15] X. Zhang and D. Zhang, in *IOP Conference Series: Materials Science and Engineering*, Vol. 108 (IOP Publishing, 2016) p. 012020.

[S16] B. Brenny, T. Coenen, and A. Polman, Journal of Applied Physics **115**, 244307 (2014).
